# Supplementary material for: Convex Relaxations for Consensus and Non-Minimal Problems in 3D Vision
Source: arXiv:1909.12034 source file (2019-09-26)
Supplement: Supplementary file 2 [file supp.tex]

\begin{proof}[Proof of Proposition~\textcolor{red}{3.2/3.3}:]
Let us define $\epsilon_i=\delta_i^2$, $\mathsf{v}=[\mathsf{x}^\intercal, \delta_1,\ldots,\delta_m ]^\intercal$,   $\mathsf{\Lambda}_0={\scriptsize\begin{bmatrix} 0&\\&\mathsf{I}_{m\times m}\end{bmatrix}}$,  $\mathsf{\Lambda}^+_i={\scriptsize\begin{bmatrix} \mathsf{G}_i&\\&\mathsf{E}^{i}\end{bmatrix}}$ and 
$\mathsf{\Lambda}^-_i={\scriptsize\begin{bmatrix} -\mathsf{G}_i&\\&\mathsf{E}^{i}\end{bmatrix}}$
with $e^{i}_{ii}=1$ and $(e^{i}_{ij})_{j\not=i}=0$. For $g_i(\mathsf{v})=z_1(\mathsf{v})^\intercal\mathsf{\Lambda}_iz_1(\mathsf{v})$,
the POP of polynomials $\{g_0(\mathsf{v}),g^+_i(\mathsf{v}),g^-_i(\mathsf{v}), i=0,\ldots m\}$
can be relaxed, similar to~(\textcolor{red}{2}), as       
\begin{equation}
\underset{\mathsf{\Upsilon}\succeq0}{\text{min}\,\,} \Big\{\text{tr}(\mathsf{\Lambda}_0\mathsf{\Upsilon})|\,\,  \text{tr}(\mathsf{\Lambda}^+_i\mathsf{\Upsilon}),
\text{tr}(\mathsf{\Lambda}^-_i\mathsf{\Upsilon})\geq 0,i=1,\ldots,m \Big\},
\label{eq:shorrlxProof}
\end{equation}
where $\text{tr}(\mathsf{\Lambda}_0\mathsf{\Upsilon}):=g_0(\mathsf{v})=\sum_i{\epsilon_i}$. We choose   $\mathsf{\Upsilon}={\scriptsize\begin{bmatrix} \mathsf{Y}&\\&\mathsf{I}_{m\times m}\end{bmatrix}}$ such that
$g_0(\mathsf{v})=\sum_i{\delta^2_i}=\sum_i{\epsilon_i}$ is satisfied.
For polynomials
$g^+_i(\mathsf{v})=z_1(\mathsf{v})^\intercal\mathsf{\Lambda}^+_iz_1(\mathsf{v})=tr(\mathsf{G}_i\mathsf{Y})-\delta^2_i$ and
$g^-_i(\mathsf{v})=z_1(\mathsf{v})^\intercal\mathsf{\Lambda}^-_iz_1(\mathsf{v})=\delta^2_i-tr(\mathsf{G}_i\mathsf{Y})$, \eqref{eq:shorrlxProof} becomes,
\begin{equation}
\underset{\mathsf{\mathsf{Y}}\succeq0}{\text{min}\,\,} \Big\{\sum_i{\delta^2_i}|\,\,  
-{\delta^2_i}\leq\text{tr}(\mathsf{G}_i\mathsf{Y})\geq {\delta^2_i},i=1,\ldots,m \Big\}.
\label{eq:shorrlxProof2}
\end{equation}
After considering $\epsilon_i=\delta_i^2$,~\eqref{eq:shorrlxProof2} becomes an SDP of~(\textcolor{red}{6/7}).
\hfill \qed
\end{proof}
